# Supplementary material for: Mixing by Unstirring: Hyperuniform Dispersion of Interacting Particles upon Chaotic Advection
Source: arXiv:1702.02395 ancillary file (2017-07-06)
Supplement: Supplementary file 1 [file SI.pdf]

# Mixing by Unstirring — Supplementary information

Joost H. Weijs[1] and Denis Bartolo[1]
[1] *Univ Lyon, Ens de Lyon, Univ Claude Bernard, CNRS, Laboratoire de Physique, F-69342 Lyon, France*

**Contents**

**I. Supplementary Videos** 1

**II. Numerical Methods** 1

**III. Characterization of the chaotic flow** 2
A. Flow field and particle dynamics 2
B. Poincaré-maps (chaotic flow) 3
C. Strobed dynamics and effective interaction range 3
D. Strobed particle dynamics 4
E. Counter-intuitive phase diagram 5

**IV. Practical considerations: Inertia** 6

**V. Scaling exponents and the effect of $L$** 6

**References** 8

## I. SUPPLEMENTARY VIDEOS

List of supplementary videos with a brief description.

- `#1` — Strobed movie (each frame at the start of a new cycle) of particle movement under AC shear flow conditions ($\gamma_0 = 3$, $\phi = 0.157$). Red circles: active particles. Blue circles: Particles with time-reversible trajectories.
- `#2` — Strobed movie (each frame at the start of a new cycle) of the particle movement under chaotic flow conditions ($\gamma_0 = 3$, $n_{\rm sub} = 3$, $\phi = 0.031$). Red circles: active particles. Blue circles: Particles with time-reversible trajectories.
- `#3` — Time evolution of the density field coarse grained at a scale $\ell = 3.5a$ starting from a uniform distribution of particles. Comparison between AC shear ($\gamma_0 = 3$) and palindromic chaotic flows ($\gamma_0 = 1$, $n_{\rm sub} = 5$). In both cases $\phi = 0.27$.
- `#4` — Time evolution of the density field coarse grained at a scale $\ell = 3.5a$ starting from a concentrated patch of particles. Comparison between: (i) AC shear ($\gamma_0 = 3$), two palindromic chaotic flows [(ii) $\gamma_0 = 3$, $n_{\rm sub} = 1$ and (iii) $\gamma_0 = 3$, $n_{\rm sub} = 3$], and (iv) the hybrid sequence described in the main text ($n_{\rm sub} = 3$ for the initial dispersion phase, $\gamma_0 = 3$ for both phases). The corresponding instantaneous exponents $\lambda(t)$ are shown for all simulations.

## II. NUMERICAL METHODS

For the simulations presented in this Letter, in order to avoid any other source of irreversibility than that due to inter-particle collisions, the arithmetic used to update particle positions as they are advected must be exactly reversible. This is particularly the case for the chaotic simulations, in which any minute perturbation is exponentially amplified. For this reason, the use of standard floating-point arithmetic is not possible. This can be clearly exemplified in the case where particles are passive tracers, where we demand that particles exactly retrace their path backwards after flow reversal (there is no physical source of irreversibility, $\epsilon = 0$). However, due to intermediate rounding (that

has to occur due to the finite precision of any stored number) there exist cases for which common mathematical truths don't hold. As an example, consider the following operation:

$$\mathrm{double}(0.1) + \mathrm{double}(0.2) - \mathrm{double}(0.2) = 0.10000000000000003331... \tag{1}$$

the result is different from

$$\mathrm{double}(0.1) = 0.10000000000000000555... \,. \tag{2}$$

Here we introduced the function double() which converts any real number to its floating-point representation in 8 bytes (IEEE 754 double precision). The operation above could represent for example the change of the $x$-coordinate of a particle as it is advected: It starts at $x = 0.1$ and due to advection it moves over 0.2 units in the positive $x$-direction. Its new location as stored in memory is then double((double(0.1) + double(0.2)). Next the flow is (precisely) reversed, hence the particle will be advected in the negative $x$-direction by an amount of double(0.2), and we find that the particle does *not* exactly return to double(0.1), as readily seen in the expanded notation above. It is important to note that this is *not* solely due to the inability to store some numbers (such as 0.1) exactly in this particular floating point standard, but happens due to the way intermediate results are rounded to a non-uniform grid of discrete representable values.

The problem may be subtle, but the solution is straight-forward: Avoid floating point arithmetic. Instead we use an integer discretization which does not suffer from these problems, as integers are naturally evenly spaced on the number line. So even though precision is of course still finite, at least the advection dynamics will be perfectly reversible. In this work, all coordinates ($\in [0,1]^2$) are discretized this way on a $2^{64} \times 2^{64}$ even grid, such that globally we do not lose precision compared to the $2 \times 64$-bit floating point representation. To test whether the use of integers indeed eliminated any added numerical irreversibility, we simulated a dense (in the sense that we're in the irreversible part of the parameter space) and highly chaotic system, setting $\epsilon = 0$ and thus eliminating any physical source of irreversibility. As expected, we found that all particles exactly retrace their steps back to their initial positions, thereby confirming that the numerics do not add any irreversible motion. This numerical scheme allows us to perform exact simulations even fro strongly chaotic flows. For sake of consistency, the same scheme is also used for simple-shear simulations.

## III. CHARACTERIZATION OF THE CHAOTIC FLOW

### A. Flow field and particle dynamics

We recall that the advection-flow field in a subcycle is given by:

$$\begin{aligned} \mathbf{v}(x,y,t) =& \gamma_0(1-|2y-1|)\hat{\mathbf{x}} && \text{for } 0 < t \ (\mathrm{mod}\ 1) < t_x \,, \\ \mathbf{v}(x,y,t) =& -\gamma_0(1-|2x-1|)\hat{\mathbf{y}} && \text{for } t_x < t \ (\mathrm{mod}\ 1) < 1 \,. \end{aligned} \tag{3}$$

Here, the all lengths have been rescaled with the size of the simulation box such that the $x$- and $y$-coordinates span from 0 to 1. This flow was chosen such that (i) no discontinuity of the velocity exists, including at the periodic boundary conditions, and (ii) that $|\nabla \mathbf{v}|$ is a constant everywhere, except at two discontinuities at the boundaries and the center lines of the simulation box. The particle dynamics resulting from passive advection is given by:

$$\dot{\mathbf{x}}_i(t) = \mathbf{v}(x_i, y_i, t) \,, \tag{4}$$

$$x_i = x_i \ (\mathrm{mod}\ 1) \,, \tag{5}$$

$$y_i = y_i \ (\mathrm{mod}\ 1) \,, \tag{6}$$

note that $\mathbf{x}_i = \begin{bmatrix} x_i \\ y_i \end{bmatrix}$.

When all ($n_{\mathrm{sub}}$) subcycles are done, the backwards phase begins, the flow is reversed and follows the same amount of subcycles such that each fluid element returns to its original location. The flow field during this phase is thus given by:

$$\begin{aligned} \mathbf{v}(t) =& \gamma_0(1-|2x-1|)\hat{\mathbf{y}} && \text{for } 0 < t \ (\mathrm{mod}\ 1) < 1 - t_x \,, \\ \mathbf{v}(t) =& -\gamma_0(1-|2y-1|)\hat{\mathbf{x}} && \text{for } 1 - t_x < t \ (\mathrm{mod}\ 1) < 1 \,. \end{aligned} \tag{7}$$

(8)

Apart from the change in direction, the order of the horizontal and vertical shear are reversed as well. In the special case where $t_x = T = 1$, there is only a flow in the $x$-direction and we thus recover a simple AC shear flow, which is not chaotic. The only other case studied in this Letter is $t_x = 0.5$, *i.e.* the case where the horizontal and vertical shear amplitudes are equal. In the following sections we characterize the chaoticity of this flow.

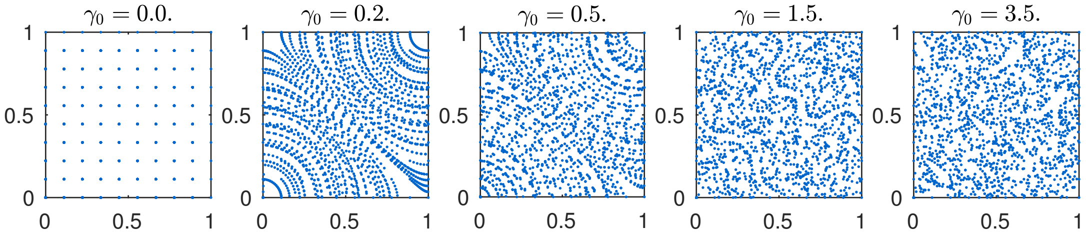


FIG. S1: Poincaré-maps of the chaotic flow [Eq. (3), $t_x = 1/2$] starting from a regular point configuration (left-most panel) at various shear amplitudes $\gamma_0$ under 20 successive mappings.

## B. Poincaré-maps (chaotic flow)

In Fig. S1 we show the advection-pattern of the chaotic flow ($t_x = 0.5$) by means of a Poincaré-map at varying shear amplitudes $\gamma_0$. The initial locations of the tracers is shown in the leftmost panel ($\gamma_0 = 0$), and is a regular pattern of $10 \times 10$ tracers. The other panels show the cumulative strobed maps after 20 subcycles at various shear amplitudes. At smaller scales and particularly for low values of $\gamma_0$ there exist clear inhomogeneities: integrable islands [*e.g.* around ($x = 0$, $y = 0$)] are surrounded by chaotic seas. The size of the islands becomes progressively smaller for larger values of $\gamma_0$. However we stress that even for finite values of $\gamma_0$, the displacements due to collisions of the particles (for finite values of $\epsilon$) promote particle escapes from the integrable regions.

## C. Strobed dynamics and effective interaction range

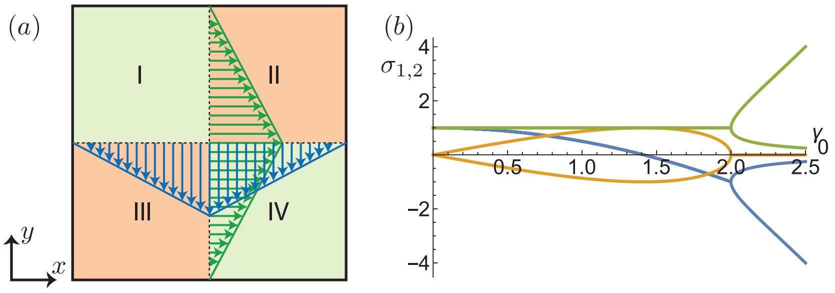


FIG. S2: (a) Horizontal and vertical shear phases superimposed, revealing the existence of four quadrants with distinctive flow characteristics. Quadrants II and III are paired through similar dynamics, where the velocity gradients of the horizontal and vertical flows are pointed either both in the positive $x$ or $y$-direction, or both in the negative $x$ or $y$-direction. For quadrants I and IV the opposite holds. (b) Eigenvalues $\sigma_{1,2}$ of $A$ [Eq. (9)] as a function of $\gamma_0$ for $t_x = \frac{1}{2}, ab < 0$ (thus, quadrants II and III). Green: $|\sigma_{1,2}|$, Blue: $\mathrm{Re}(\sigma_{1,2})$, and orange: $\mathrm{Im}(\sigma_{1,2})$. For this value of $t_x$, a Hopf-like bifurcation exists at $\gamma_0 = 2$. For the case $ab > 0$ which represent quadrants I and IV and is not shown here the flow is hyperbolic for any value of $\gamma_0$, *i.e.* $\max(|\sigma_{1,2}(\gamma_0)|) > 1$.

The irreversible dynamics in the simulations are fully determined by the *relative* motion of the advected particles with respect to each other, as only this motion can put two particles in contact leading to an irreversible event (namely, a collision and the corresponding kick $\epsilon$). This relative motion is especially useful to study the separation dynamics of two particles that start close together, hence quantifying the effective interaction range as described in the main text.

Let us study the relative motion of a pair of particles in terms of a discrete mapping. The position of one particle relative to another particles maps to a new relative position after one subcycle as follows:

$$\begin{bmatrix} x_{t+1} \\ y_{t+1} \end{bmatrix} = \begin{bmatrix} 1 & a \\ b & 1+ab \end{bmatrix} \begin{bmatrix} x_t \\ y_t \end{bmatrix} = A \begin{bmatrix} x_t \\ y_t \end{bmatrix}, \tag{9}$$

where $a = t_x\gamma_0$ in quadrants III and IV shown in Fig. S2(a), and $a = -t_x\gamma_0$ in quadrants I and II. Furthermore, $b = (1-t_x)\gamma_0$ in quadrants II and IV and $b = -(1-t_x)\gamma_0$ in quadrants I and III. There are therefore two types of flow in this map, one type occurs in quadrants I and IV ($ab < 0$), the other in II and III ($ab > 0$): In the case of quadrants I and IV, the velocity gradient during the horizontal shear phase and during the vertical shear phase are of the same sign with respect to the vertical ($y$) and horizontal ($x$) coordinates leading to a hyperbolic mapping as the square of the trace of $A$ is always larger than 4 for non-zero $\gamma_0$. Contrarily in quadrants II and III the velocity gradients are not of the same sign among the horizontal and vertical shear phasess, thus $ab < 0$ meaning that the mapping is non-hyperbolic as $\mathrm{tr}^2(A) < 4$. As we will see, for low enough values of $\gamma_0$ particles will enter stable orbits relative to each other leading to integrable trajectories.

When looking more closely at the properties of the mapping $A$, we see first of all that the determinant of $A$ is always equal to 1:

$$|A(a,b)| = 1\ . \tag{10}$$

This is to be expected as the mapping is a composite of two subsequent shear operations both of which are area-preserving. The composite mapping is therefore area preserving.

Secondly, we study the eigenvalues of $A$:

$$\sigma_{1,2} = 1 + \frac{ab \pm \sqrt{ab(4+ab)}}{2}\ . \tag{11}$$

We use the letter $\sigma$ to indicate eigenvalues instead of the usual $\lambda$ to avoid confusion with the hyperunformity exponent $\lambda$. Here we see that the sign of $ab$ is crucial. In quadrants I and IV, where the sign of $ab$ is positive, the flow is always hyperbolic: The argument under the square root is always positive for finite $\gamma_0$, and therefore the largest eigenvalue is always larger than 1, as the fraction gives a value greater than 0. Conversely, in the case where $ab < 0$ (quadrants II and III) there exists a Hopf-type bifurcation at $ab = -4$, or:

$$\gamma_0^H = \sqrt{\frac{4}{t_x - t_x^2}}, \tag{12}$$

where the eigenvalues become complex for any value of $\gamma_0 < \gamma_0^H$. For $t_x = 1$ (the simple shear flow) this criterium does not apply, and for the chaotic case studied in the paper ($t_x = \frac{1}{2}$) we find $\gamma_0^H = 4$. The case $t_x = \frac{1}{2}$ is displayed in Fig. S2(b), clearly showing the Hopf-bifurcation occuring at $\gamma_0 = 4$.

To compute the shape of the effective interaction region of a particle as introduced in the main text, we first compute the interaction region of a single horizontal shear operation in a similar way as was done in [1]. Taking $\Delta x$ and $\Delta y$ to be the relative distance of the particle pair in the $x$- and $y$-directions resp., the interaction region is defined there where:

$$\begin{gathered} \Delta x^2 + \Delta y^2 \le a^2\ ,\ \text{or} \\ \Delta y^2 \le a^2 \text{ and } \left|\Delta x \pm \sqrt{a^2 - \Delta y^2}\right| \le |t_x\gamma_0\Delta y|\ ,\ \text{provided that}\, \mathrm{sgn}(\Delta x) \ne \mathrm{sgn}(\Delta y)\ . \end{gathered} \tag{13}$$

Here, sgn() is the signum function. The first line in Eq. (13) signifies the region where particles already overlap at the start of the cycle, the second line are the (partial) butterfly wings as described in [1], and signify the collisions that somewhere during the shear cycle. To compute the interaction region after $n_{\mathrm{sub}}$ successive subcycles, we apply the transformation $A^{n_{\mathrm{sub}}}$ [Eq. (9)] to this region. Even though $A$ is area preserving, the area of the interaction area *does* grow with $n_{\mathrm{sub}}$ as a new 'butterfly' [Eq. (13)] is injected after each subcycle. The area therefore grows approximately linearly, whereas the extent of the extrema of the interaction region (which are the extreme of the first injected butterfly) grow exponentially when $A$ is hyperbolic.

### D. Strobed particle dynamics

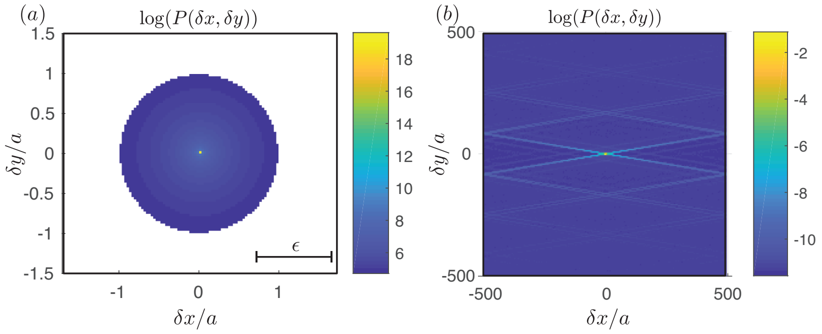


FIG. S3: Logarithms of the probability density distribution of the strobed particle displacements ($P(\delta x, \delta y)$) over 1 full cycle. For both simulations the particle density is $n = 15 \cdot 10^{-3}/a^2$ ($N = 15000$) and $\epsilon = 0.5$ which correspond to $f_\mathrm{a} = 0.3$ in both cases. (a) Discrete random-organization model, using an interaction region shown in the inset . It is identical to that found in chaotic simulations and shown in Fig. 3h in the main text. Active particles are kicked in a random direction of maximum magnitude $\epsilon$, as directly reflected by this isotropic distribution. The peak at $(\delta x, \delta y) = (0, 0)$ indicates particles that are inactive, and therefore by definition are stationary. (b) Continuous time model, as used in the paper. Here we see that particle displacements can be very large. Note the very different scales on the axes between (a) and (b)].

We now emphasize that the effect of the chaotic flow is two-fold: (i) As shown in the previous section, it causes the interaction area to be exponentially stretched with the number of subcycles, (ii) after a collision, the separation of particle trajectories is exponentially amplified. Due to the latter, the dynamics between a 'traditional' (*i.e.* discrete) random organization model and the continuous time model used in this work are qualitatively different. In other words, one cannot reproduce the results using a discrete model which employs the interaction region as defined above, and shown in Fig. S3 and Fig. 3h in the main text.

We demonstrate this result by comparing a random-organization simulation with the model used in this paper keeping the interaction region shown in the inset of Fig. S3 identical. In particular, we look at the probability density distribution of the strobed displacements of the particles over a single cycle. The discrete random organization result is the simplest to interpret. We see in Fig. S3a that all displacements are located within a disk of radius $\epsilon$ with a peak at $(\delta x, \delta y) = (0, 0)$ and a $1/r$-distribution up to $r = \epsilon$ otherwise. This is not surprising considering how the random organization model is defined: When a particle lies within the interaction region of another particle, they both experience a random kick of magnitude bounded by $\epsilon$, thereby leading to the observed isotropic distribution. The peak in the center represents the fraction of inactive particles.

The reason the result for the continuous time model (Fig. S3b) is so different is that particles that experience a random kick upon collision separate from their unperturbed trajectories in an exponential fashion. This behavior cannot be captured in a discrete time model by a mere redefinition of the particle shape. This important difference is the reason why the simulations in this work have to be performed using more expensive continuous time simulations.

From this we can conclude that: (i) The chaotic model does not merely reduce to a random organization model with an adapted interaction region. (ii) The radical change in dynamics caused by the chaoticity of the flow is responsible for the fast dispersion which is the desirable property that we aim at combining with hyperuniform organization.

### E. Counter-intuitive phase diagram

In Fig. 2f, in the main text, we found that, for a given particle fraction, increasing the noise amplitude $\epsilon$ results in a transition from an irreversible to a reversible dynamics. This phase behavior is all the more counterintuitive that the random kicks of amplitude $\epsilon$ are the only source of irreversibility in the particle dynamics. We do not have an explanation for this behaviour, it might be however worth noting a similarly counterintuitive behavior when external noise is added to conventional random organization processes [2]. Adding noise was indeed show to further increase hyperuniform organization.

We also stress here that the phase diagram reported in Fig. 2f characterizes the steady state of the driven system and is *not* a mere transient artifact. This results is clearly illustrated by Fig. S4a. The variations of the fraction of active particles is plotted as a function of time for a series of different values of $\epsilon$, keeping all other parameters constant. In all simulations the system has clearly reached a statistically stationary state over more than a thousand of cycles. The corrsponding asymptotic values of $f_a$ are plotted as a function of $\epsilon$ in Fig. S4b and clearly show a sharp transition from an irreversible to a resersible dynamics.

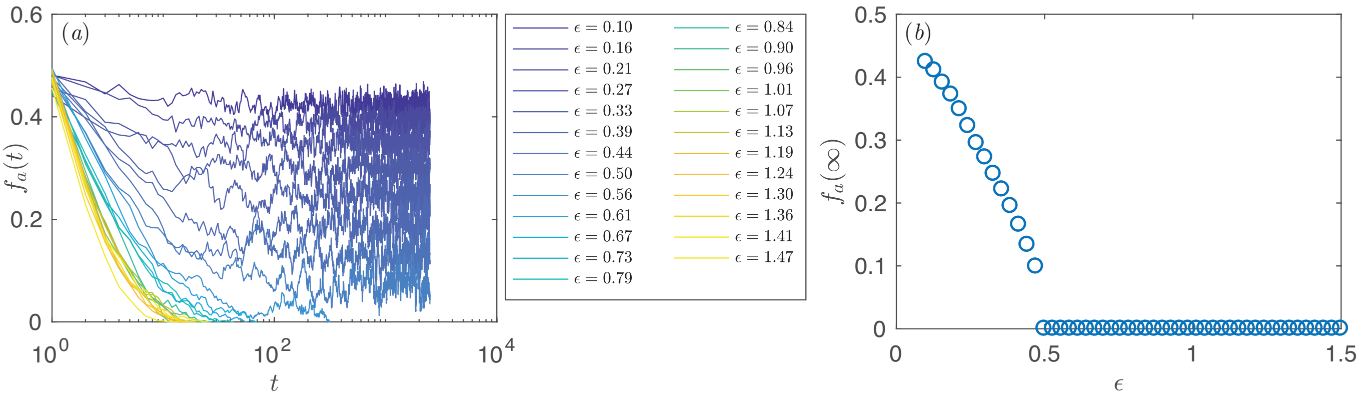


FIG. S4: Variation of reversibility for chaotical driving dynamics at varying $\epsilon$. $\phi = 3.5 \cdot 10^{-3}$, $\gamma_0 = 3$, $N = 3\,000$, and $n_{\mathrm{sub}} = 10$ (a) Time evolution of the active fraction of particles $f_a(t)$. (b) Steady state value of the active fraction of particles $f_a^\infty(\epsilon)$.

## IV. PRACTICAL CONSIDERATIONS: INERTIA

Throughout this work we have implicitly neglected particle inertia, and have therefore assumed their instantaneous response to any change in the imposed flowfield. In this section we discuss the range of application of this hypothesis. The equation of motion for such a particle is given as:

$$\ddot{\mathbf{x}} = \frac{\gamma}{m} \left( \mathbf{v}(\mathbf{x}, t) - \dot{\mathbf{x}} \right), \tag{14}$$

where $\mathbf{v}(\mathbf{x}, t)$ is the local fluid velocity, and $\mathbf{x}$, $\dot{\mathbf{x}}$, $\ddot{\mathbf{x}}$ the particle's position and its time-derivatives. For spherical particles in a viscous fluid we use Stokes' drag such that $\gamma = 6\pi\eta a$, and $m = \frac{4}{3}\rho\pi a^3$. The typical relaxation time for the particle velocity is:

$$\tau_p = \frac{m}{\gamma} = 2\frac{\rho a^2}{9\eta}. \tag{15}$$

Thus, for any real application one would have to make sure that the typical timescale at which the driving flow changes is larger than $\tau_p$. For particles with a radius of $\sim 10\,\mu$m dispersed in water, and having a very high specific weight (10 times that of water), particle inertia becomes relevant only when flow variations occur at the millisecond scale. Millimeter-size particles of density close to that of water suspended in a viscous liquid with $\eta = 10^{-1}$ mPa.s would have similar limitations. Given the large strains required for mixing, any mechanically-imposed flow, e.g. by rheometers or beaters, would clearly be associated with much slower time variations (of the order of 0.1 s at the fastest).

## V. SCALING EXPONENTS AND THE EFFECT OF $L$

The (ir)reversibility transition that occurs for non-chaotic driving flows is critical, in ref. [3] it has been extensively studied for a similar out-of-equilibrium system where the critical exponents have been determined. Here, we verify that our model (which is continuous as opposed to discrete in time in [3]) falls under the same universality class. Due to the higher computational costs associated with continuous-time simulations, the statistics are less extensive yet sufficient to conclude. In addition we perform this analysis at various box sizes $L$, to properly account for finite size effects.

First, in Fig. S5 we look at the relaxation time (towards steady state) of the system as the area fraction $\phi$ is varied around the transition. Each curve (and therefore each color) signifies a different value of the simulation box size $L$. We observe that there exists a clear maximum for all curves around $\phi \approx 0.195$. The exact location and the height of this maximum clearly depends on $L$, which is expected due to finite size effects in the vicinity of a critical point.

In Fig. S6 a systematic decrease towards $\phi^\star_{L\to\infty} = 0.195 \pm 0.002$ (95% confidence bounds, obtained by fitting to the function $\phi^\star_L = c\phi^{-1/\nu} + \phi^\star_\infty$) is observed, giving us the value of the critical density $\phi^\star$. This fit allows us to collapse the locations of the peak of $\tau$ for all values of $L$, as shown in Fig. S7 (left).

From this we can also extract the exponent $z\nu$ associated with the relaxation time for each simulation size ($\tau \sim |\phi - \phi^\star|^{-z\nu}$), as is done in Fig. S7 (right). We find values of $z\nu$ comprised between 1 and 1.4 which are consistent with the directed percolation universality class in 2D: $z\nu^{\mathrm{DP}} = 1.30$. Our data are therefore in correspondence, but

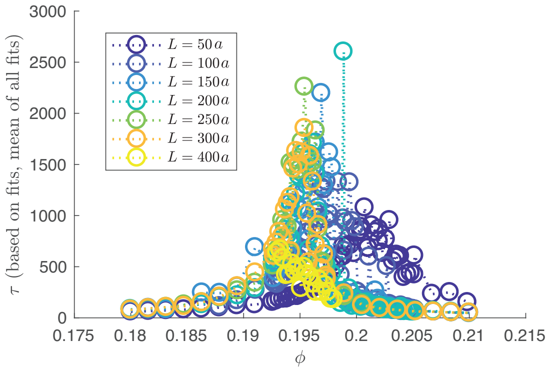


FIG. S5: Relaxation time $\tau$ as a function of area fraction $\phi$ at various system sizes $L$. To improve statistics, multiple realizations were done for all but the largest box sizes. Critical slowing down is observed to occur near the transition. The value of $\phi$ at which the apparent transition occurs, is shifted as the box-size becomes smaller due to finite size effects.

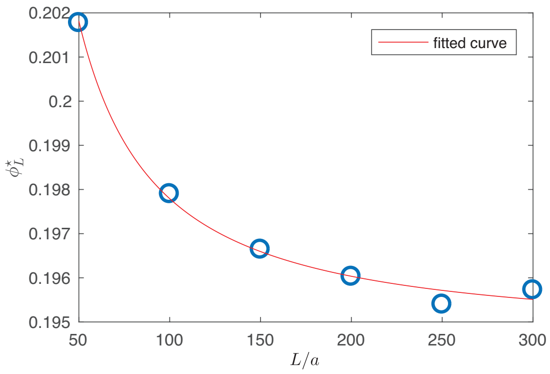


FIG. S6: Location of the peak of $\tau$ (Fig. S5) as the box size is increased including power law fit. Extrapolating the fit to $L \to \infty$ gives $\phi^\star = 0.195$.

not accurate enough to distinguish between Directed Percolation and Conserved Directed Percolation, for which $z\nu^{\mathrm{CDP}} = 1.23$.

The final exponent we measure is the one associated with the growth of the order parameter $f_a$ with the control parameter $\phi$, as shown in Fig. S8 (left). For a critical transition $f_a \sim (\phi - \phi^\star)^\beta$, and in Fig. S8(right) we see that the order parameter indeed follows a power law with an exponent $\beta = 0.56$ for large $L$, which is closer to Directed Percolation ($\beta^{\mathrm{DP}} = 0.58$) than Conserved Directed Percolation ($\beta^{\mathrm{CDP}} = 0.64$).

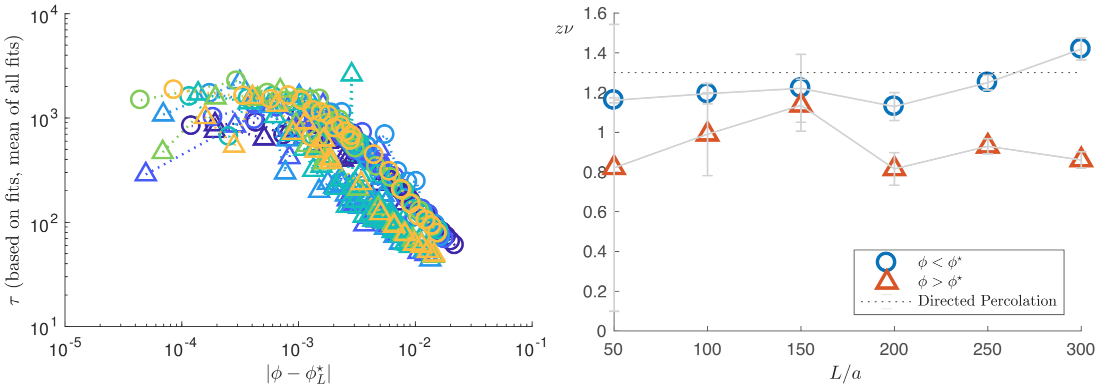


FIG. S7: Left: Log-log plot of reshifted curves of $\tau$ (cf. Fig. S6). Right: Fitted exponents, giving $z\nu$

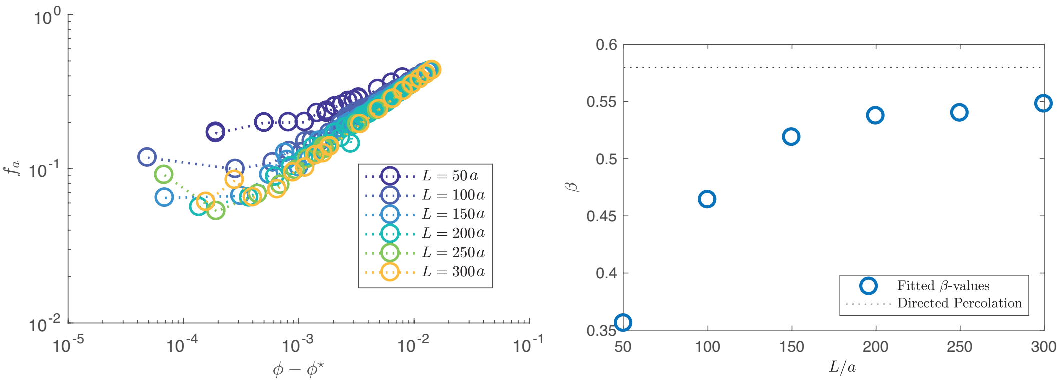


FIG. S8: Left: Shifted $f_a(\phi)$-curves on a log-log scale. The curves clearly follow a power-law behaviour, with exponent $\beta$. Right: Fitted exponent $\beta$ for various values of $L$. As $L$ becomes larger (and finite size effects diminishes) the value of the exponent approaches that known for the directed percolation universality class: $\beta^{\mathrm{DP}} = 0.58$.

[1] K. J. Schrenk and D. Frenkel, The Journal of Chemical Physics **143**, 241103 (2015).
[2] D. Hexner and D. Levine, Phys. Rev. Lett. **118**, 020601 (2017).
[3] E. Tjhung and L. Berthier, J. Stat. Mech. Theor. Exp. **2016**, 033501 (2016).
